# Supplementary material for: SparseFusion: Distilling View-conditioned Diffusion for 3D Reconstruction
Source: arXiv:2212.00792 source file (2023-02-15)
Supplement: Supplementary file 1 [file 6-supplementary.tex]

% % CVPR 2023 Paper Template
% % based on the CVPR template provided by Ming-Ming Cheng (https://github.com/MCG-NKU/CVPR_Template)
% % modified and extended by Stefan Roth (stefan.roth@NOSPAMtu-darmstadt.de)

% \documentclass[10pt,twocolumn,letterpaper]{article}

% %%%%%%%%% PAPER TYPE  - PLEASE UPDATE FOR FINAL VERSION
% \usepackage[review]{cvpr}      % To produce the REVIEW version
% % \usepackage{cvpr}              % To produce the CAMERA-READY version
% %\usepackage[pagenumbers]{cvpr} % To force page numbers, e.g. for an arXiv version

% % Include other packages here, before hyperref.
% \usepackage{graphicx}
% \usepackage{amsmath}
% \usepackage{amssymb}
% \usepackage{booktabs}

% % generic util file that ST likes
% \usepackage{lib}

% %#################
% %##CUSTOM ZZZ 
% %#################
% \usepackage{bm}
% \usepackage[table]{xcolor}
% \usepackage{stmaryrd}
% \usepackage{multirow}
% \newcommand\TODO[1]{\textcolor{red}{\textbf{[TODO: #1]}}}
% \newcommand{\outline}[1]{\textcolor{purple}{#1}}
% \newcommand{\znote}[1]{\textcolor{blue}{Z: #1}}
% \newcommand{\parnobf}[1]{\vspace{1mm} \par \noindent {\bf {#1}}}
% % \usepackage[compact]{titlesec}
% % \titlespacing{\section}{0pt}{2ex}{1ex}
% % \titlespacing{\subsection}{0pt}{1ex}{0ex}
% % \titlespacing{\subsubsection}{0pt}{0.5ex}{0ex}

% % It is strongly recommended to use hyperref, especially for the review version.
% % hyperref with option pagebackref eases the reviewers' job.
% % Please disable hyperref *only* if you encounter grave issues, e.g. with the
% % file validation for the camera-ready version.
% %
% % If you comment hyperref and then uncomment it, you should delete
% % ReviewTempalte.aux before re-running LaTeX.
% % (Or just hit 'q' on the first LaTeX run, let it finish, and you
% %  should be clear).
% \usepackage[pagebackref,breaklinks,colorlinks]{hyperref}
% \usepackage{epigraph}

% \input{macros}


% % Support for easy cross-referencing
% \usepackage[capitalize]{cleveref}
% \crefname{section}{Sec.}{Secs.}
% \Crefname{section}{Section}{Sections}
% \Crefname{table}{Table}{Tables}
% \crefname{table}{Tab.}{Tabs.}


% %%%%%%%%% PAPER ID  - PLEASE UPDATE
% \def\cvprPaperID{7031} % *** Enter the CVPR Paper ID here
% \def\confName{CVPR}
% \def\confYear{2023}


% \begin{document}

% %%%%%%%%% TITLE - PLEASE UPDATE
% \title{
% Supplementary Materials:\\SparseFusion: Distilling View-conditioned Diffusion for 3D Reconstruction
% }


% % \maketitle
% \twocolumn[{
% \maketitle
% }]

% %%%%%%%%%%%%%%%%%%%%%%%%%%%%%%%
% %%%%%%%%%% INTRO TEXT %%%%%%%%%
% %%%%%%%%%%%%%%%%%%%%%%%%%%%%%%%
% We provide a more detailed overview of denoising diffusion probabilistic models. We provide implementation details for each component our approach, epipolar feature transformer (EFT), View-conditioned Diffusion Model (VLDM), and diffusion distillation. We include a web page to visualize 360 degree renderings in \textbf{\emph{index.html}}. Finally, we provide a narrated video of our approach in  \textbf{\emph{sparsefusion\_overview.mp4}}.

% %%%%%%%%%%%%%%%%%%%%%%%%%%%%%%%
% %%%%%%%%%% BODY TEXT %%%%%%%%%%
% %%%%%%%%%%%%%%%%%%%%%%%%%%%%%%%
% \input{supp/supp-a.tex}
% \input{supp/supp-b.tex}
% \input{supp/supp-c.tex}

% %%%%%%%%%%%%%%%%%%%%%%%%%%%%%%%
% %%%%%%%%% REFERENCES %%%%%%%%%%
% %%%%%%%%%%%%%%%%%%%%%%%%%%%%%%%
% {\small
% \bibliographystyle{ieee_fullname}
% \bibliography{egbib}
% }

% \end{document}
