# Supplementary material for: SparseFusion: Distilling View-conditioned Diffusion for 3D Reconstruction
Source: arXiv:2212.00792 source file (2023-02-15)
Supplement: Supplementary file 2 [file supp-b.tex]

%%%%%%%%%%%%%%%%%%%%%%%%%%%%%%%
%%%%%%%%%% More Results %%%%%%%%%%%
%%%%%%%%%%%%%%%%%%%%%%%%%%%%%%%

\section{Additional Experiments}
\seclabel{more-results}

\paragraph{Ablation on Diffusion Distillation.}
\input{supp/supp-ablations.tex}
We examine the performance of various diffusion distillation setups in \tableref{supp-ablation}. We study the effects of three design choices: the loss space, the number of denoising steps, and whether perceptual loss is used. We observe that for all methods, PSNR remain relatively similar. However, computing loss in pixel space and using perceptual loss improves SSIM and LPIPS. Moreover, we find that performing multiple denoising steps leads to the best perceptual results while balancing the three quantitative metrics.
